# Supplementary material for: On the Relation between Sensitivity and Accuracy in In-context Learning
Source: arXiv:2209.07661 source file (2024-01-27)
Supplement: Supplementary file 1 [file tab_sensitivity_corr_appendix.tex]

\begin{table*}[t]
\fontsize{9.5}{9.5}\selectfont
% \small
\setlength{\tabcolsep}{3pt}
\centering
\begin{tabular}{llccccccccccc}
\toprule
Adj. & Perturb & AG News & ARP & DBP & Emo & CARER & WikiQA & YAT & LYR & YRFS & MR & Avg \\
\cmidrule{2-13}
\multirow{3}{*}{None} & Inst - H & $\text{-0.438}^\dagger$ & $\text{-0.440}^\dagger$ & $\text{-0.203}^\dagger$ & $\text{-0.228}^\dagger$ & -0.156 & -0.113 & -0.149 & $\text{-0.424}^\dagger$ & $\text{-0.183}^\dagger$ & $\text{-0.328}^\dagger$ & -0.266 \\
\cmidrule{2-13}
& Inst - A & $\text{-0.272}^\dagger$ & $\text{-0.327}^\dagger$ & -0.167 & -0.089 & -0.111 & -0.302 & -0.192 & $\text{-0.343}^\dagger$ & $\text{-0.084}^\dagger$ & -0.157 & -0.204 \\
\cmidrule{2-13}
& Ex Ord & $\text{-0.145}^\dagger$ & $\text{-0.358}^\dagger$ & $\text{-0.159}^\dagger$ & $\text{\textbf{-0.295}}^\dagger$ & -0.080 & / & -0.132 & $\text{-0.590}^\dagger$ & $\text{-0.215}^\dagger$ & $\text{-0.322}^\dagger$ & -0.255 \\
\midrule
\multirow{3}{*}{CC} & Inst - H & $\text{\textbf{-0.501}}^\dagger$ & $\text{\textbf{-0.577}}^\dagger$ & $\text{-0.571}^\dagger$ & $\text{-0.097}^\dagger$ & $\text{\textbf{-0.359}}^\dagger$ & $\text{\textbf{-0.515}}^\dagger$ & $\text{-0.385}^\dagger$ & $\text{-0.472}^\dagger$ & $\text{-0.253}^\dagger$ & $\text{-0.336}^\dagger$ & -0.407 \\
\cmidrule{2-13}
& Inst - A & -0.228 & -0.269 & $\text{-0.382}^\dagger$ & $\text{0.000}$ & -0.136 & $\text{-0.391}^\dagger$ & $\text{-0.280}^\dagger$ & $\text{-0.328}^\dagger$ & $\text{-0.161}^\dagger$ & $\text{-0.370}^\dagger$ & -0.254 \\
\cmidrule{2-13}
& Ex Ord & $\text{-0.191}^\dagger$ & $\text{-0.484}^\dagger$ & $\text{-0.516}^\dagger$ & $\text{-0.282}^\dagger$ & $\text{-0.240}^\dagger$ & $\text{-0.310}^\dagger$ & $\text{-0.301}^\dagger$ & $\text{-0.567}^\dagger$ & $\text{-0.194}^\dagger$ & $\text{-0.419}^\dagger$ & -0.350 \\
\midrule
\multirow{3}{*}{PC} & Inst - H & $\text{-0.491}^\dagger$ & $\text{-0.541}^\dagger$ & $\text{-0.688}^\dagger$ & $\text{-0.274}^\dagger$ & $\text{-0.351}^\dagger$ & $\text{-0.065}^\dagger$ & $\text{-0.393}^\dagger$ & $\text{\textbf{-0.624}}^\dagger$ & $\text{-0.256}^\dagger$ & $\text{\textbf{-0.542}}^\dagger$ & \textbf{-0.422} \\
\cmidrule{2-13}
& Inst - A & $\text{-0.427}^\dagger$ & $\text{-0.445}^\dagger$ & $\text{-0.646}^\dagger$ & $\text{-0.269}^\dagger$ & $\text{-0.315}^\dagger$ & $\text{-0.185}^\dagger$ & $\text{\textbf{-0.540}}^\dagger$ & $\text{-0.507}^\dagger$ & $\text{-0.238}^\dagger$ & $\text{-0.337}^\dagger$ & -0.391 \\
\cmidrule{2-13}
& Ex Ord & $\text{-0.381}^\dagger$ & $\text{-0.459}^\dagger$ & $\text{\textbf{-0.822}}^\dagger$ & -0.159 & $\text{-0.333}^\dagger$ & -0.089 & $\text{-0.503}^\dagger$ & $\text{-0.518}^\dagger$ & $\text{\textbf{-0.258}}^\dagger$ & $\text{-0.471}^\dagger$ & -0.399 \\
\bottomrule
\end{tabular}
\caption{\label{tab:sensitivity-corr-rawcc} The correlation between the sensitivity and accuracy of ICL predictions. We observe that sensitivity is negatively correlated with accuracy, with stronger correlation when decision boundary adjustment methods are applied to mitigate label bias. $^\dagger$ denotes correlations with $p$-value $< 0.05$. %Inst - H: human instruction perturbations. Inst - A: automatic instruction perturbations. Ex Ord: example ordering perturbations.
}
\end{table*}
